# Supplementary material for: Floquet formulation of the dynamical Berry-phase approach to non-linear optics in extended systems
Source: arXiv:2208.10213 ancillary file (2023-04-10)
Supplement: Supplementary file 1 [file SupplementalMaterial.pdf]

# Supplemental Material

## Floquet formulation of the dynamical Berry-phase approach to non-linear optics in extended systems

Ignacio M. Alliati[1] and Myrta Grüning[1,*]

[1]*School of Mathematics and Physics, Queen's University Belfast, Belfast BT7 1NN, Northern Ireland, United Kingdom*

### I. COMPUTATIONAL COST

In this section, we present the actual computational cost of each run, rather than the RT-to-FL ratio shown in Fig. 7 and 8 of the manuscript. The format of these figures is the same as Fig. 7 and 8 for comparability.

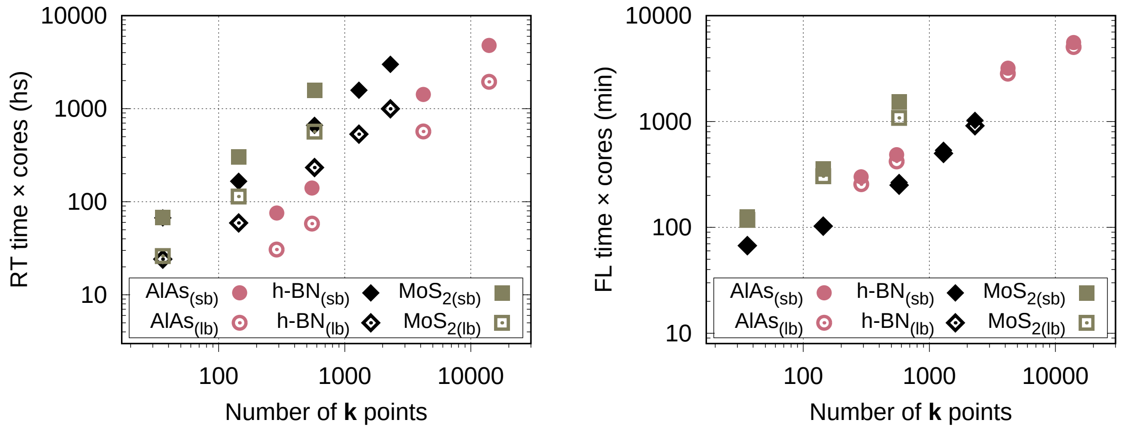


FIG. S1: Computational cost of SHG calculations in CPU time multiplied by the number of cores.

*Also at European Theoretical Spectroscopy Facility (ETSF)

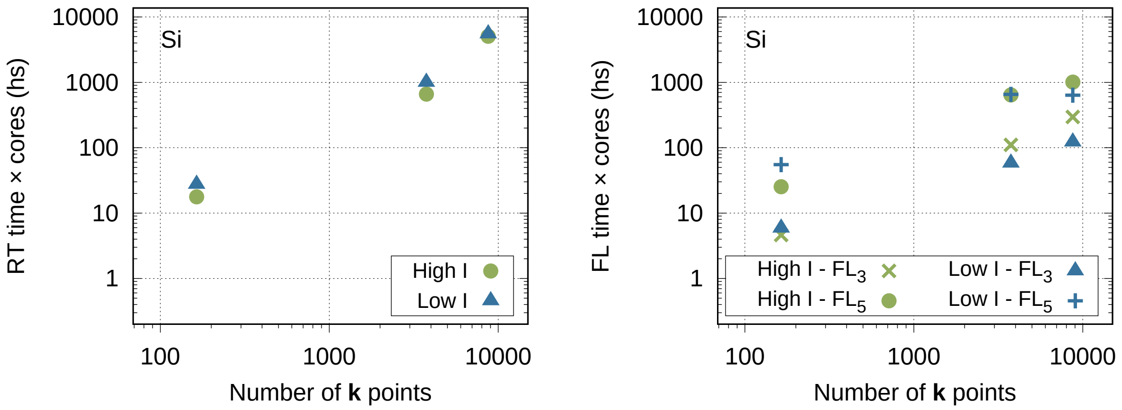


FIG. S2: Computational cost of THG calculations in CPU time multiplied by the number of cores.

## II. FLOQUET SCALING

We present the scaling of the calculation time of our approach with respect to the number of Floquet modes. Bulk AlAs with a $20\times20\times20$ **k**-grid was taken as an example. The data is produced *via* a first-order Floquet calculation with $\eta_{\max} = 1 - 6$, i.e., with $0 - 5$ extra Floquet modes. The data is presented as CPU time per iteration per frequency, so it is representative of calculating the Hamiltonian matrix, diagonalising it, calculating the polarisation and extracting the Fourier coefficients. The near-quadratic scaling reflects the diagonalisation time, since the size of the Hamiltonian at a given **k**-point is $N_{bands} \times (2\,\eta_{\max} + 1)$. This operation is performed using the QR-algorithm, i.e., what is usually referred to as full diagonalisation.

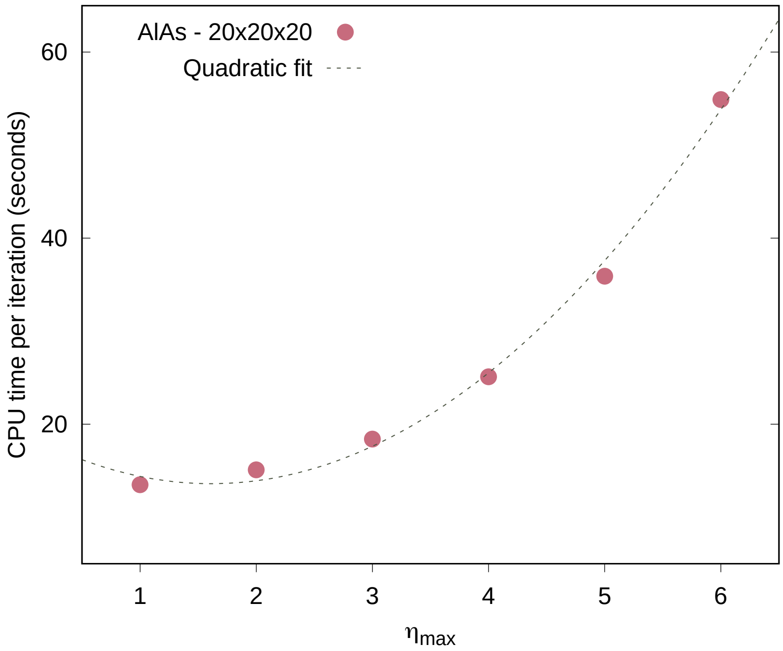


FIG. S3: Scaling with Floquet modes - CPU time per iteration per frequency

## III. COMPUTATIONAL DETAILS

The DFT calculations were performed with Quantum Espresso (QE) 6.7. The real-time (RT) and Floquet calculations were done with a developer branch of Yambo 5.1 where we incorporated our formalism. The details for these calculations are as show in Tables S1 and S2.

See next section for the determination of the real-time convergence parameters.

| | AlAs | h-BN | $MoS_2$ |
|---|---|---|---|
| Calculated spectra | LR, SHG | LR, SHG | LR, SHG |
| **k**-grids (scf) | 10×10×10 | 12×12×1 | 12×12×1 |
| **k**-grids (nscf) | 8×8×8, | 6×6×1, | 6×6×1, |
| | 10×10×10, | 12×12×1 | 12×12×1, |
| | 20×20×20, | 24×24×1 | 24×24×1, |
| | 30×30×30 | 36×36×1 | |
| | | 48×48×1 | |
| Bands (full–empty) | 3–6 | 4–4 | 5–5 |
| Band-gap correction [eV] | 0.9 | 3.3 | 0.72 |
| Broadening [eV] (sb;lb) | 0.04; 0.15 | 0.04; 0.15 | 0.04; 0.15 |
| Total time [fs] (sb;lb) | 118; 48 | 235; 83 | 230; 85 |
| Time step [as] | 10 (2.5) | 2.5 | 10 |
| Intensity [kW/cm$^2$] | $1 \times 10^3$ | $1 \times 10^3$ | $1 \times 10^3$ |
| Floquet modes $\eta_{\max}$ | 2 | 2 | 2 |

TABLE S1: Computational details of the SHG data set. The acronyms sb and lb stand for small and large broadening, respectively.

| | Si |
|---|---|
| Calculated spectra | THG |
| **k**-grids (scf) | 8×8×8 |
| **k**-grids (nscf) | 8×8×8 |
| | 24×24×24 |
| | 32×32×32 |
| Bands (full–empty) | 4–3 |
| Band-gap correction [eV] | 0.6 |
| Broadening [eV] | 0.15 |
| Total time [fs] | 74 |
| Time step [as] | 10 |
| Intensity [kW/cm$^2$] (lI;hI) | $1 \times 10^3$; $1 \times 10^7$ |
| Floquet modes $\eta_{\max}$ (lI;hI) | 3; 5 |

TABLE S2: Computational details of the THG data set. The acronyms lI and hI stand for low and high intensity, respectively.

## IV. CONVERGENCE REAL-TIME

The real-time convergence parameters reported in the previous section were chosen on the basis of the following convergence tests. They are all performed on the coarse grid for each material. SHG convergence tests for the dephasing time are done with 0.04 eV (small broadening) and 0.15 eV (large broadening). SHG convergence tests for the time step are done only at small broadening. THG convergence tests are done only at large broadening, and also at two different intensities, namely $1 \times 10^3$ (low intensity) and $1 \times 10^7$ (high intensity) kW/cm$^2$. These convergence tests allow us to determine the time step and dephasing time required for each calculation, as shown in Tables S1 and S2.

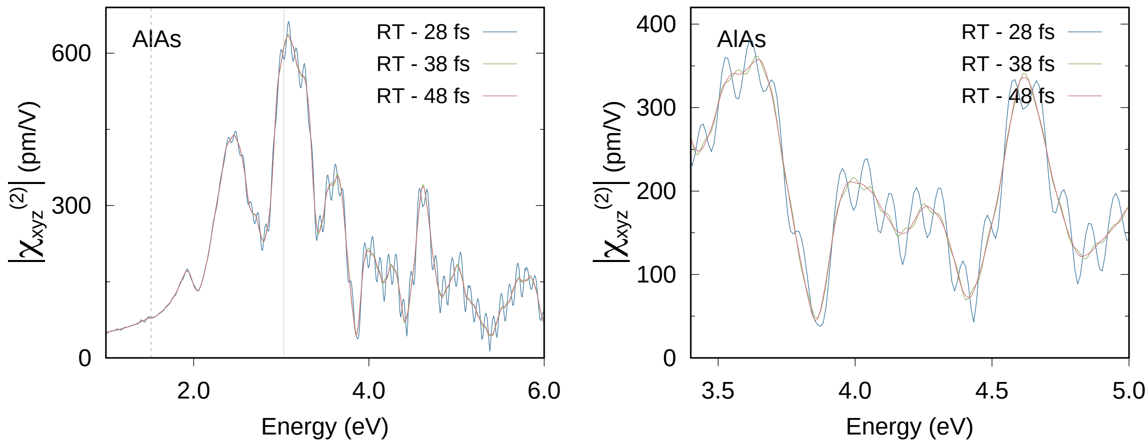


FIG. S4: Bulk AlAs - dephasing time - large broadening

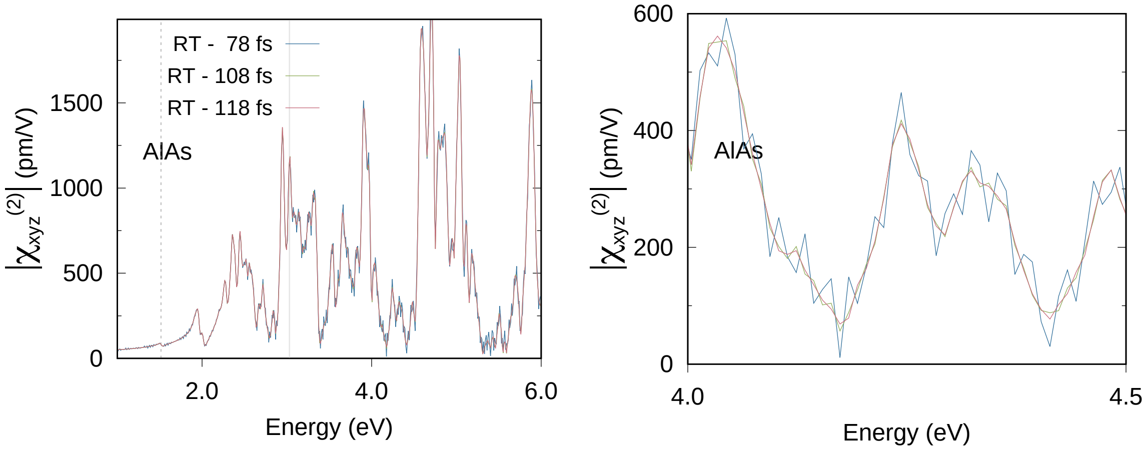


FIG. S5: Bulk AlAs - dephasing time - small broadening

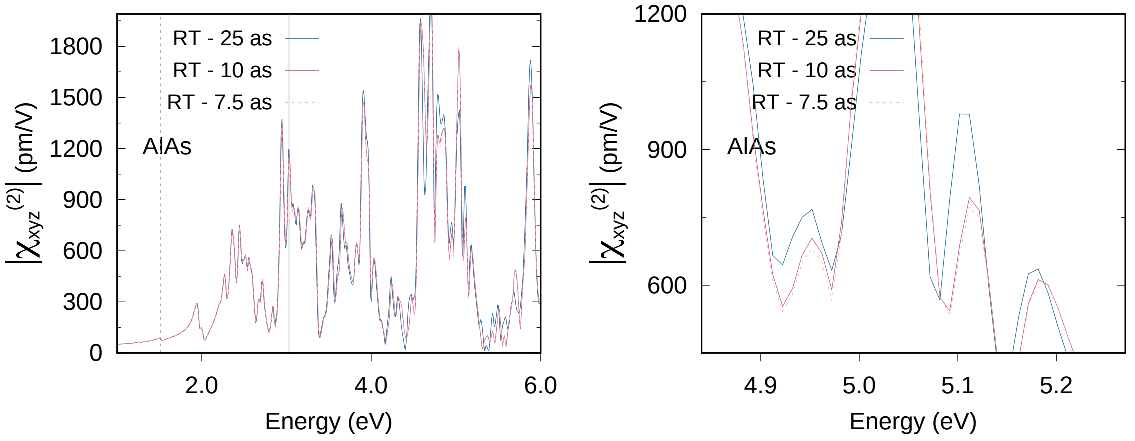


FIG. S6: Bulk AlAs - time step - small broadening

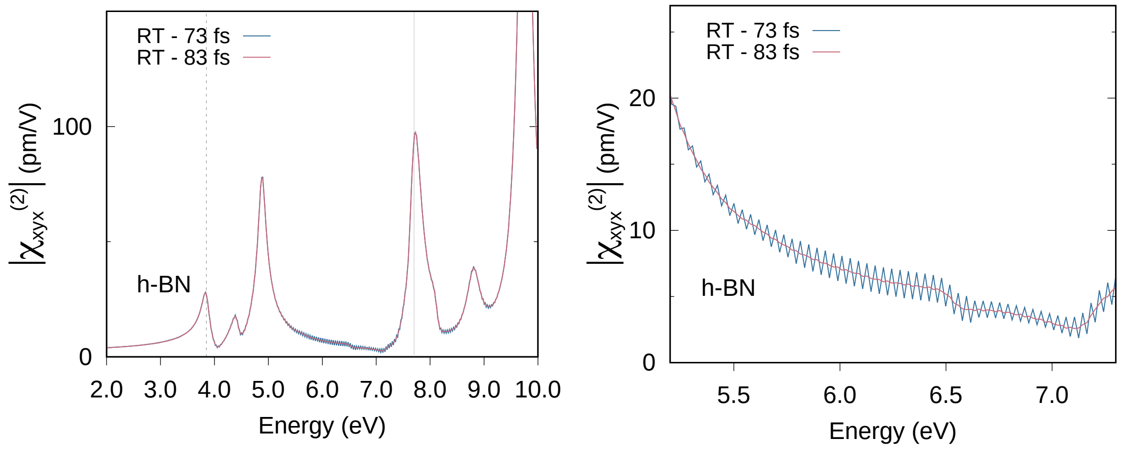


FIG. S7: h-BN 2D - dephasing time - large broadening

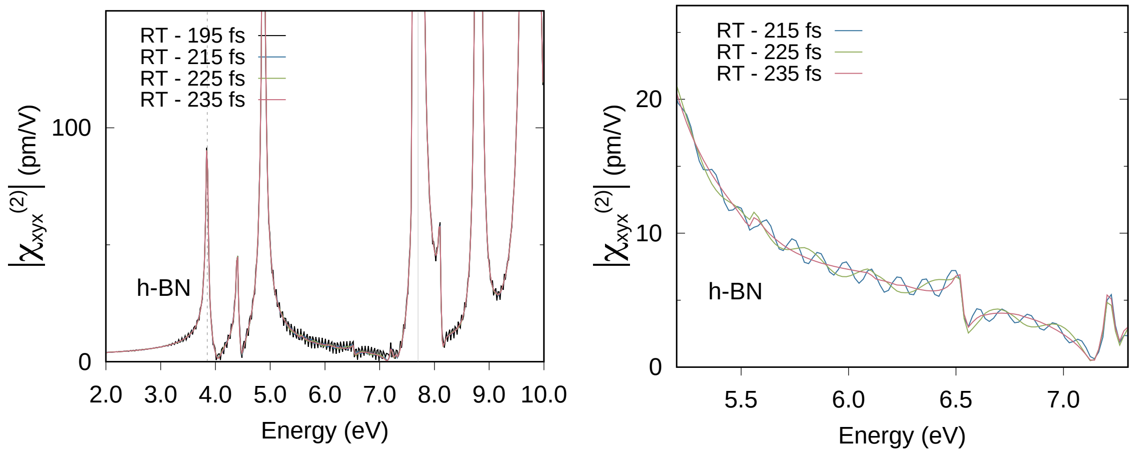


FIG. S8: h-BN 2D - dephasing time - small broadening

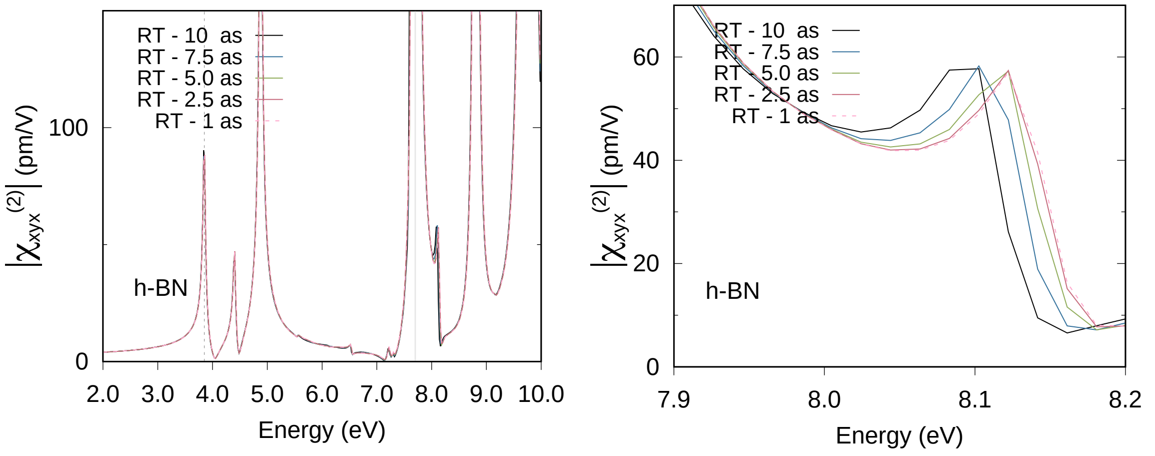


FIG. S9: h-BN 2D - time step - small broadening

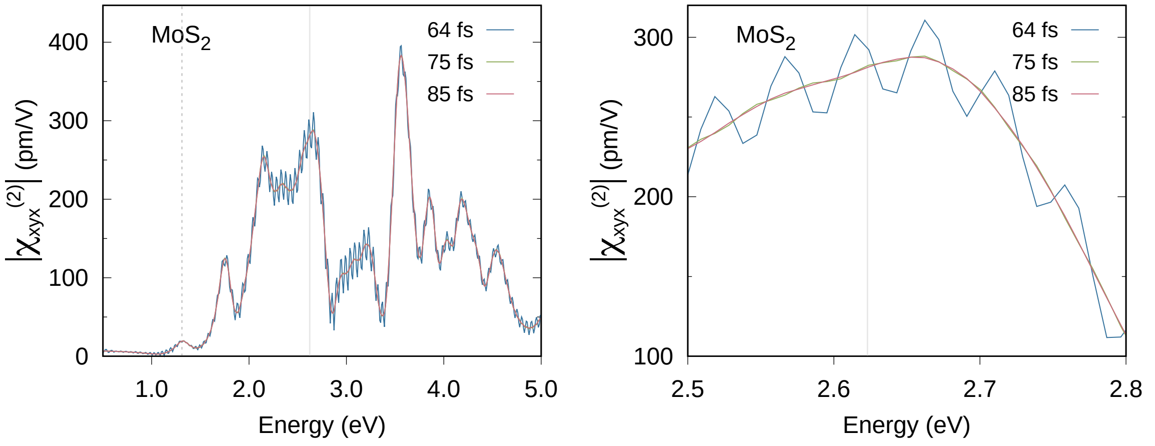


FIG. S10: $MoS_2$ 2D - dephasing time - large broadening

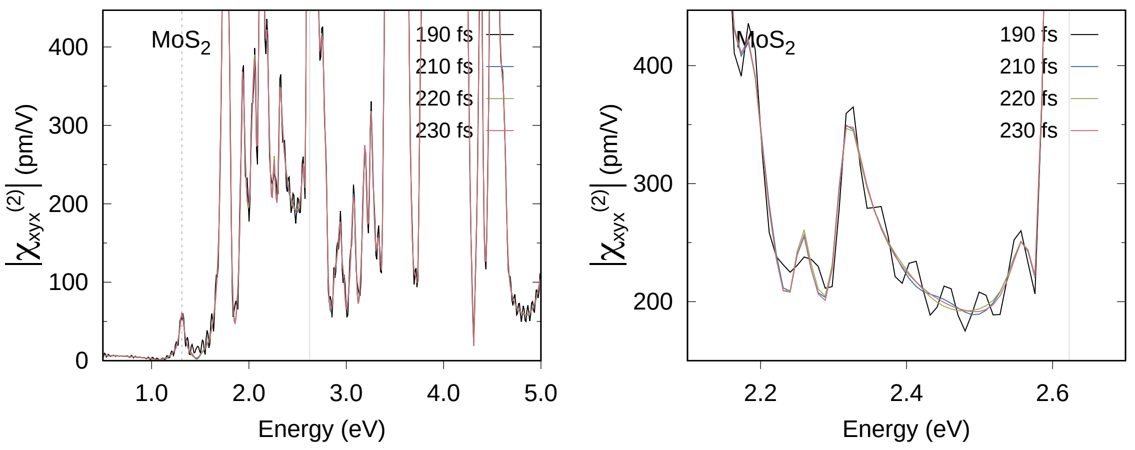


FIG. S11: $MoS_2$ 2D - dephasing time - small broadening

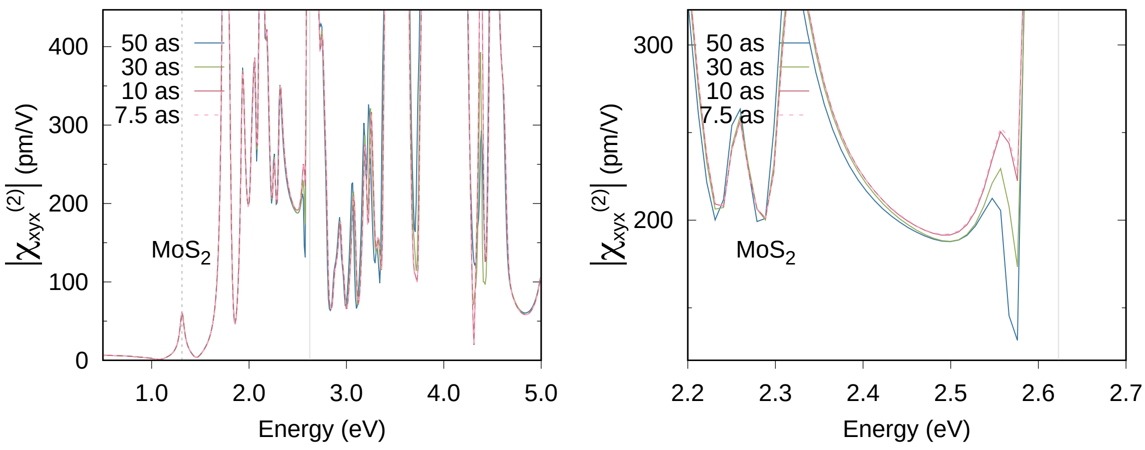


FIG. S12: $MoS_2$ 2D - time step - small broadening

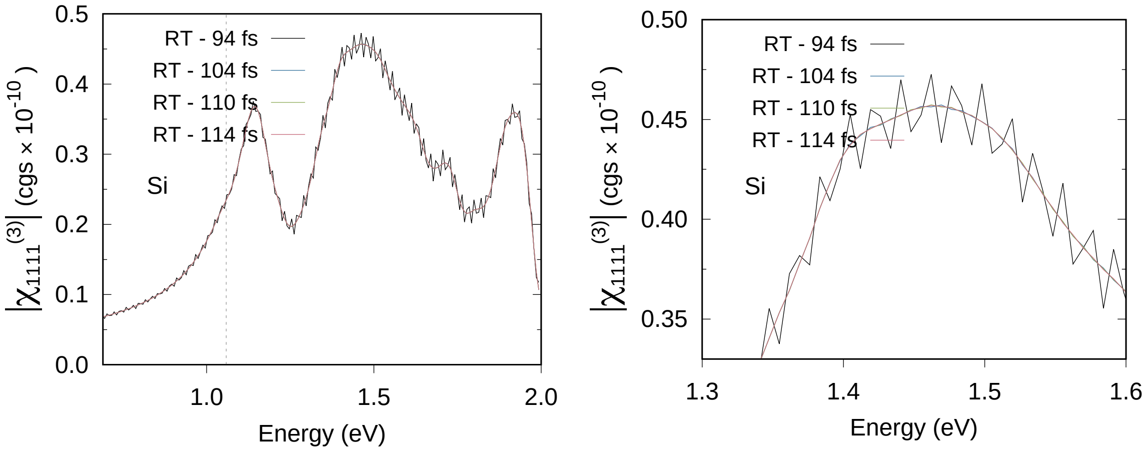


FIG. S13: Si bulk THG - dephasing time - low intensity

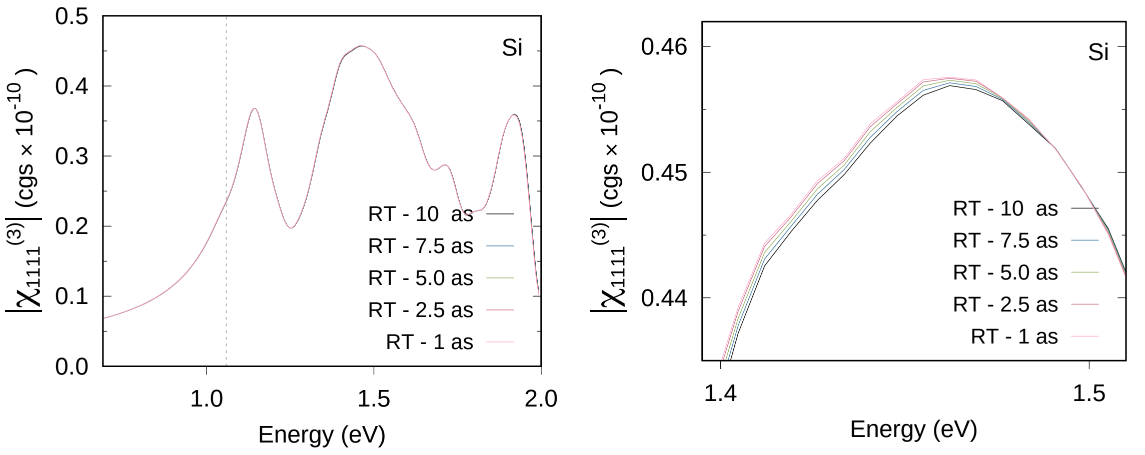


FIG. S14: Si bulk THG - time step - low intensity

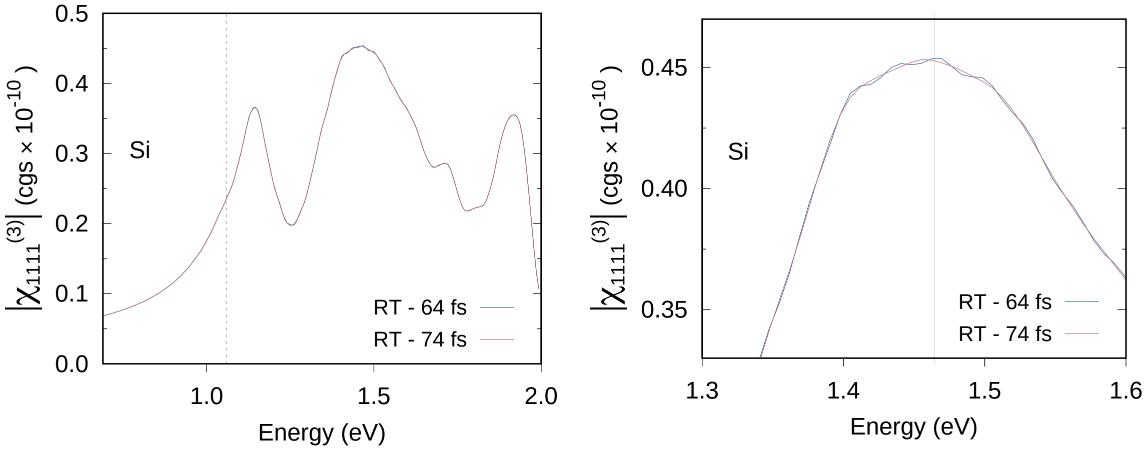


FIG. S15: Si bulk THG - dephasing time - high intensity

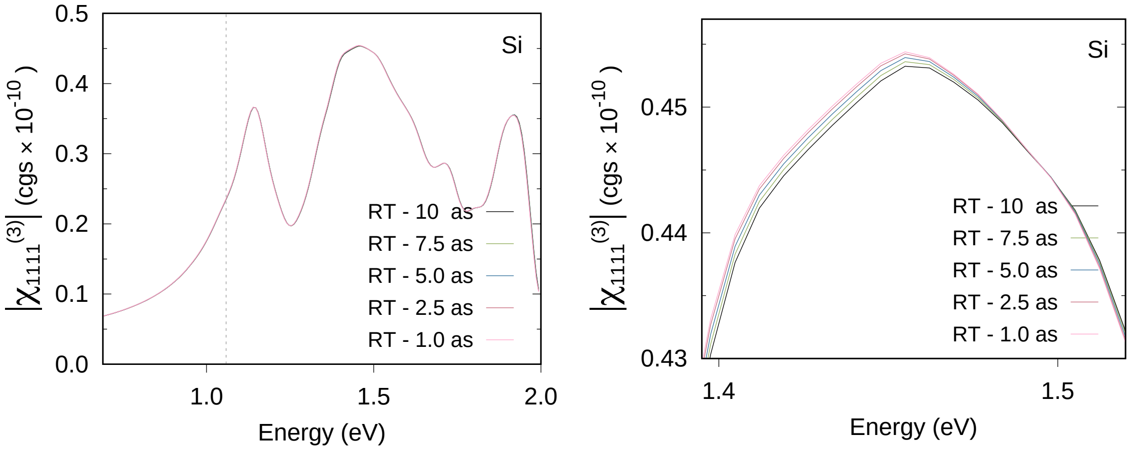


FIG. S16: Si bulk THG - time step - high intensity

## V. CONVERGENCE FLOQUET

Convergence of our Floquet approach with respect to the number of Floquet modes is reported in this section. We present tests for AlAs, h-BN and $MoS_2$ with regards to their SHG spectra, which were all performed on the coarse grid for each material (convergence for THG spectra in bulk Si is covered in the manuscript). We present data for $\eta_{\max} = 2$ ($FL_2$), $\eta_{\max} = 3$ ($FL_3$) and $\eta_{\max} = 4$ ($FL_4$). In addition to the electric-field intensity used to study SHG in the manuscript (i.e. $1 \times 10^3$ kW/cm$^2$, labelled low intensity), we report convergence tests at a higher intensity, where higher-order contributions to the second order response are expected to be important. This higher intensity is $1 \times 10^7$ kW/cm$^2$ for AlAs and h-BN, and $1 \times 10^5$ kW/cm$^2$ for $MoS_2$ since convergence issues appeared above this value. We did all our low intensity tests with a low broadening of 0.04 eV, however we had to raise it for some of the high intensity cases to improve convergence (mentioned in caption where applicable).

The results show that convergence with respect to the number of Floquet modes in the calculation of SHG spectra is very fast. Even at high intensities, higher-order contributions to SHG do not seem to have a big effect in the response and $\eta_{\max} = 2$ appears to be enough.

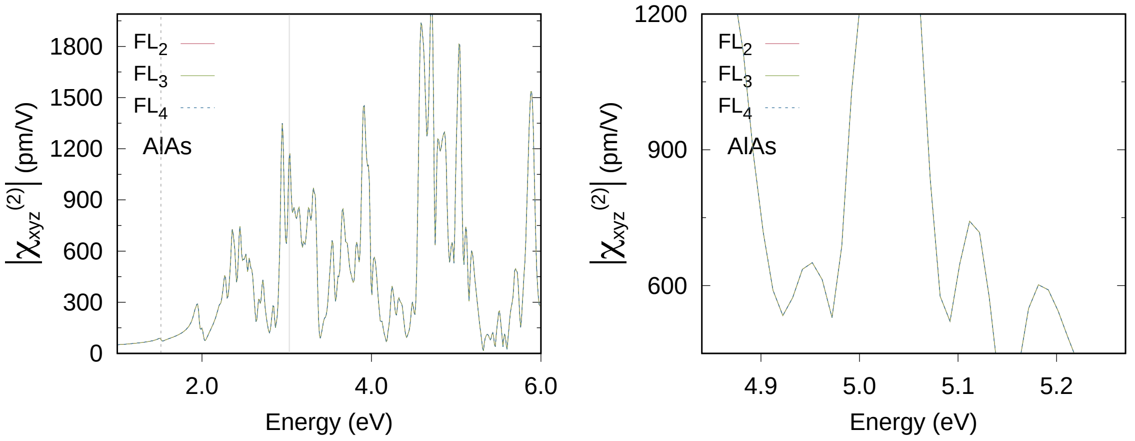


FIG. S17: AlAs bulk - Floquet modes - low intensity - 0.04 eV

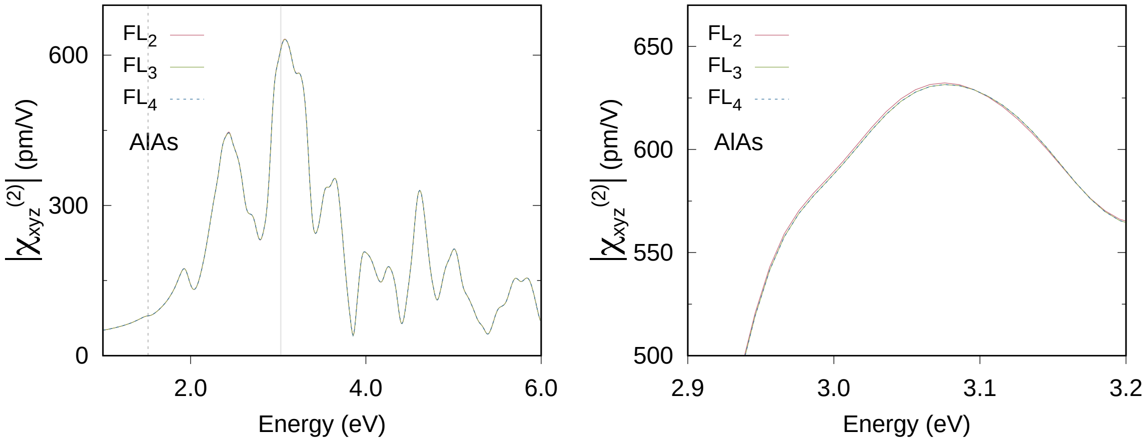


FIG. S18: AlAs bulk - Floquet modes - high intensity - 0.15 eV

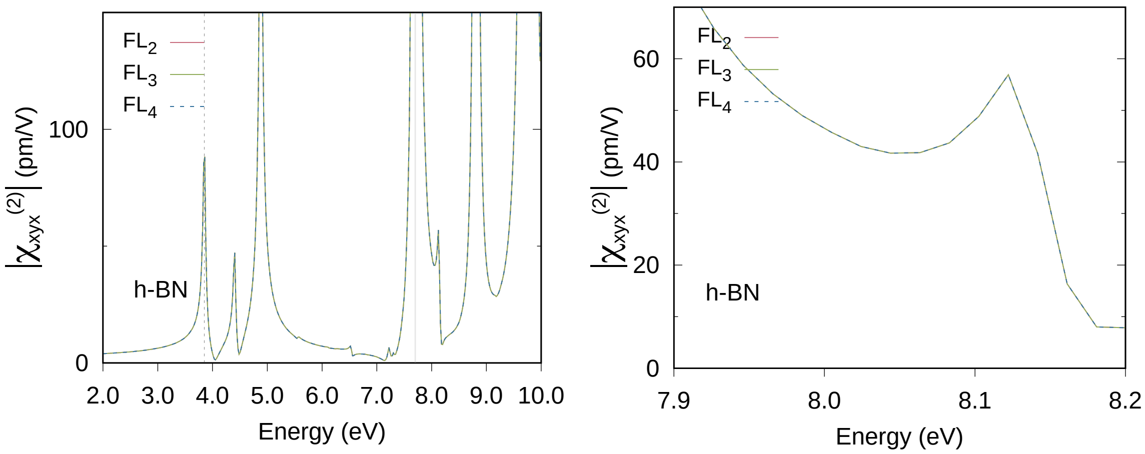


FIG. S19: h-BN 2D - Floquet modes - low intensity - 0.04 eV

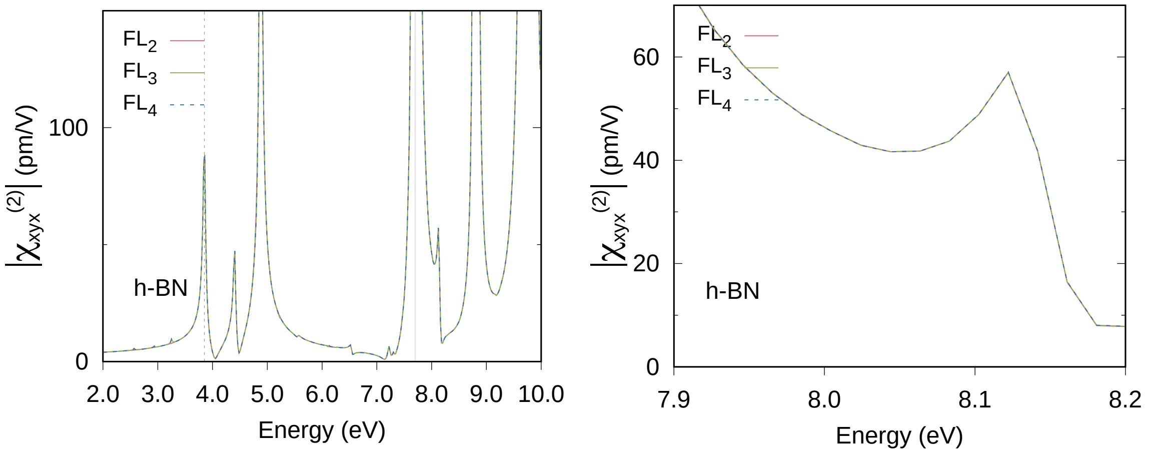


FIG. S20: h-BN 2D - Floquet modes - high intensity - 0.04 eV

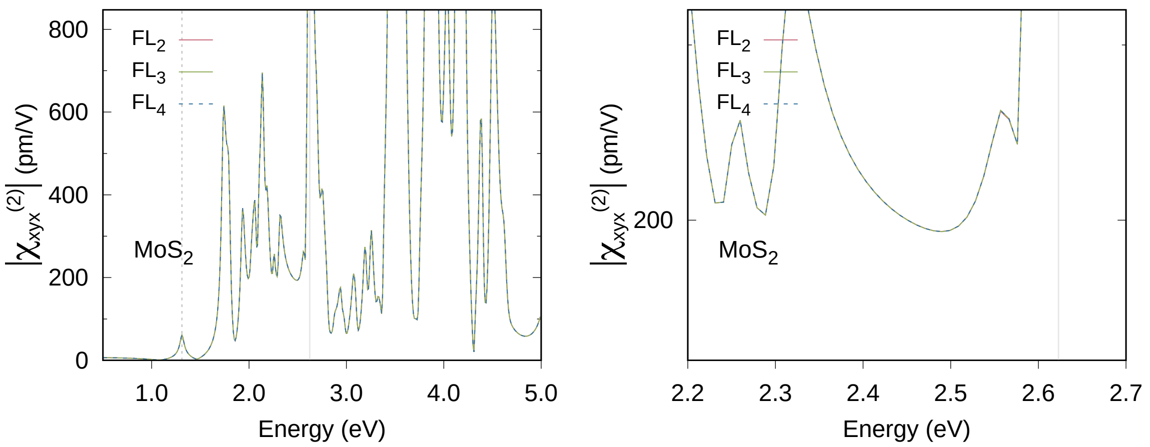


FIG. S21: $MoS_2$ 2D - Floquet modes - low intensity - 0.04 eV

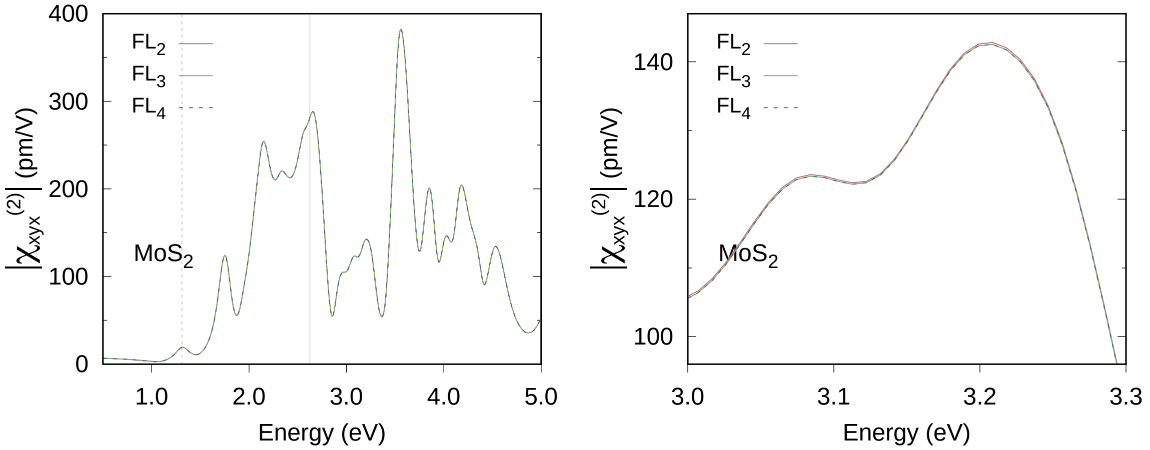


FIG. S22: $MoS_2$ 2D - Floquet modes - high intensity - 0.15 eV

## VI. RESULTS

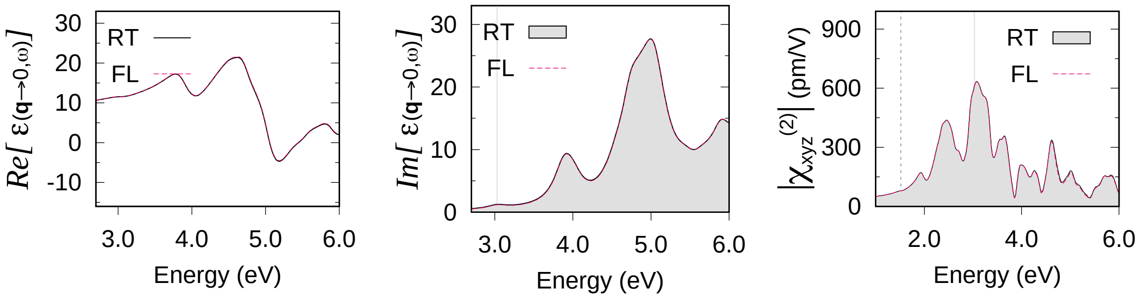


FIG. S23: Bulk AlAs - 8×8×8 - large broadening

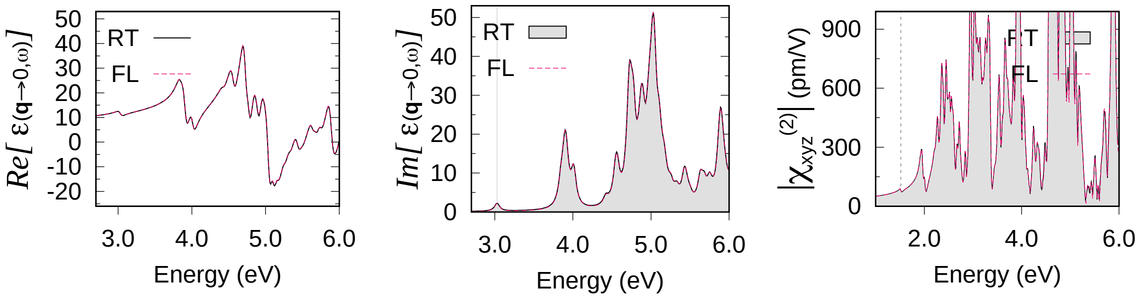


FIG. S24: Bulk AlAs - 8×8×8 - small broadening

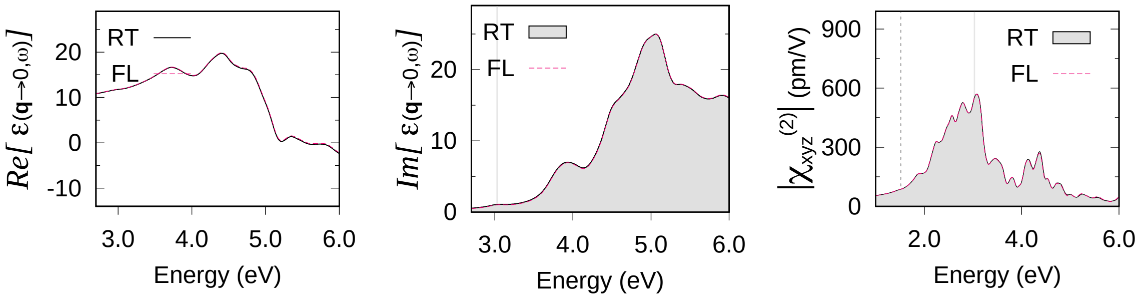


FIG. S25: Bulk AlAs - 10×10×10 - large broadening

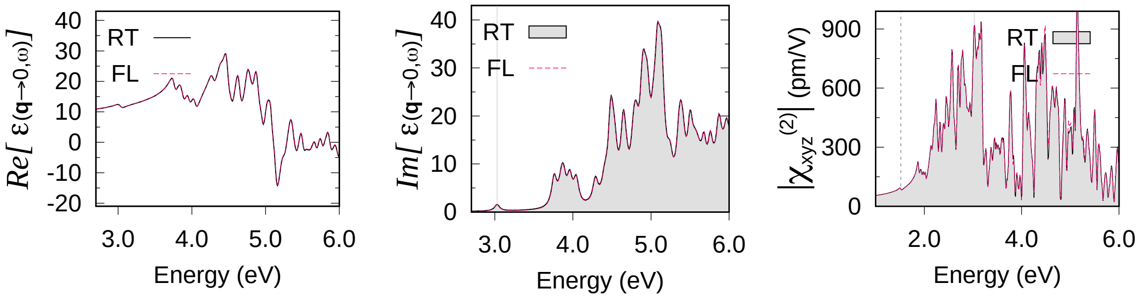


FIG. S26: Bulk AlAs - 10×10×10 - small broadening

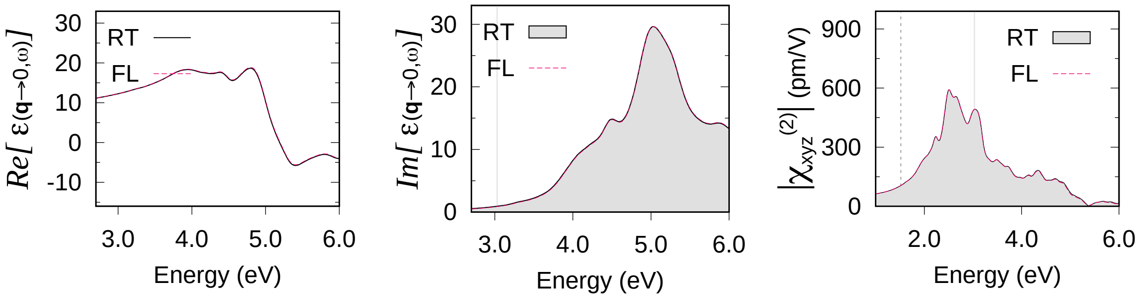


FIG. S27: Bulk AlAs - 20×20×20 - large broadening

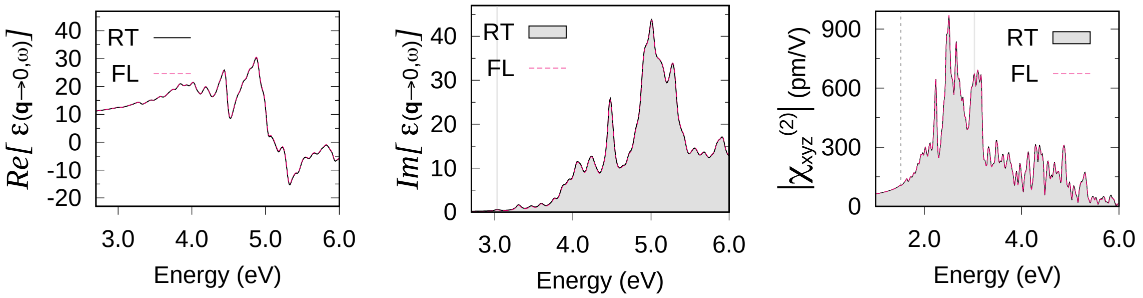


FIG. S28: Bulk AlAs - 20×20×20 - small broadening

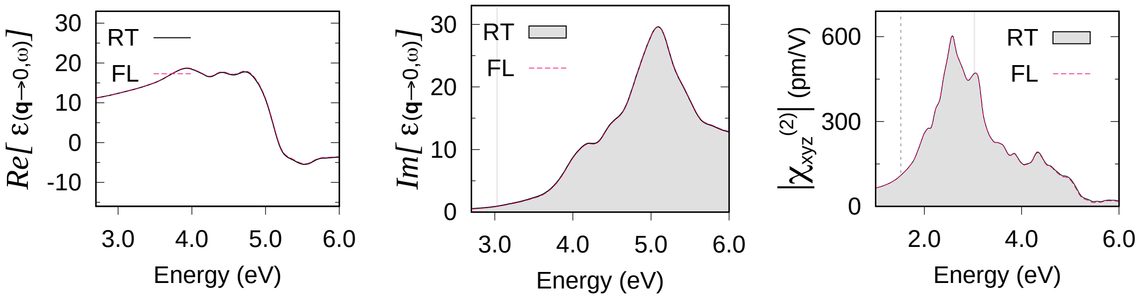


FIG. S29: Bulk AlAs - 30×30×30 - large broadening

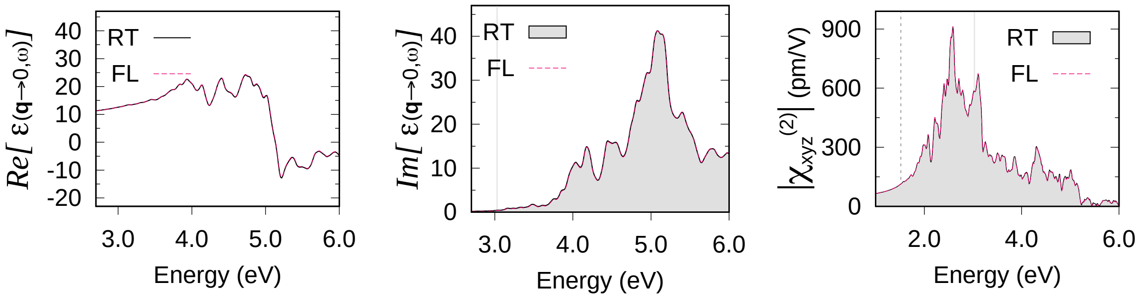


FIG. S30: Bulk AlAs - 30×30×30 - small broadening

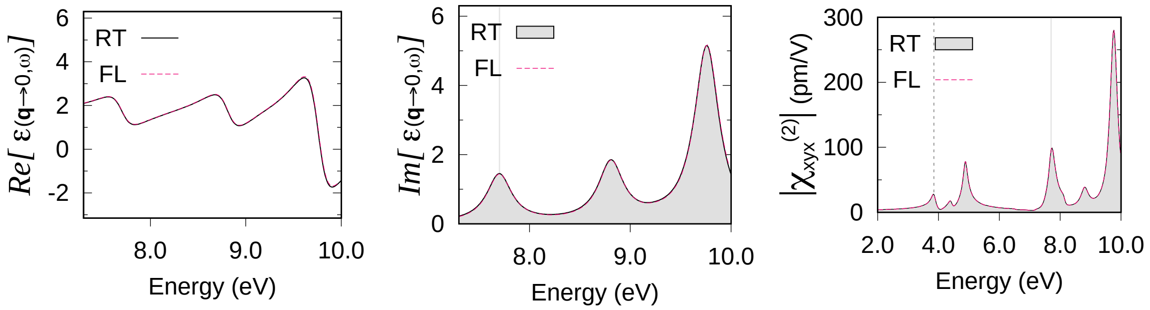


FIG. S31: h-BN 2D - 6×6×1 - large broadening

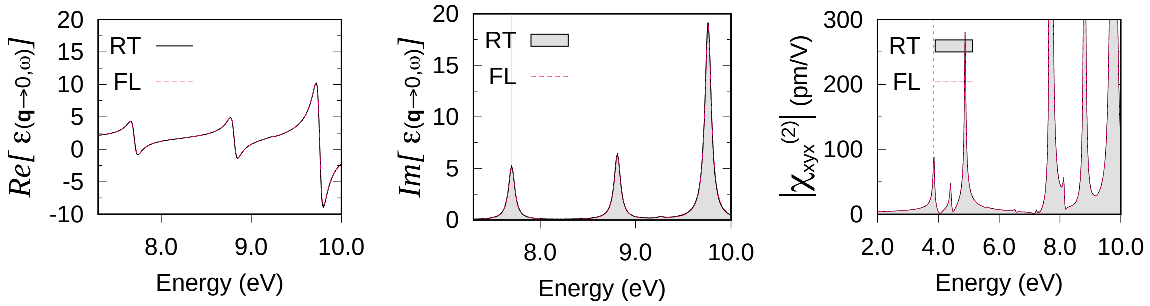


FIG. S32: h-BN 2D - 6×6×1 - small broadening

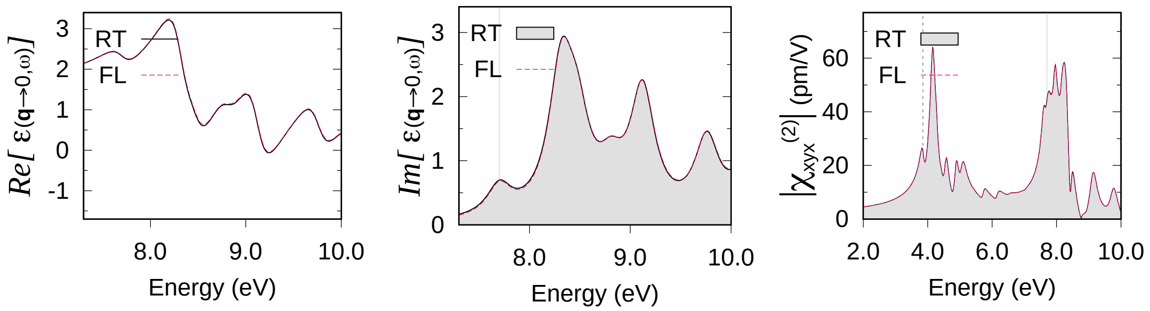


FIG. S33: h-BN 2D - 12×12×1 - large broadening

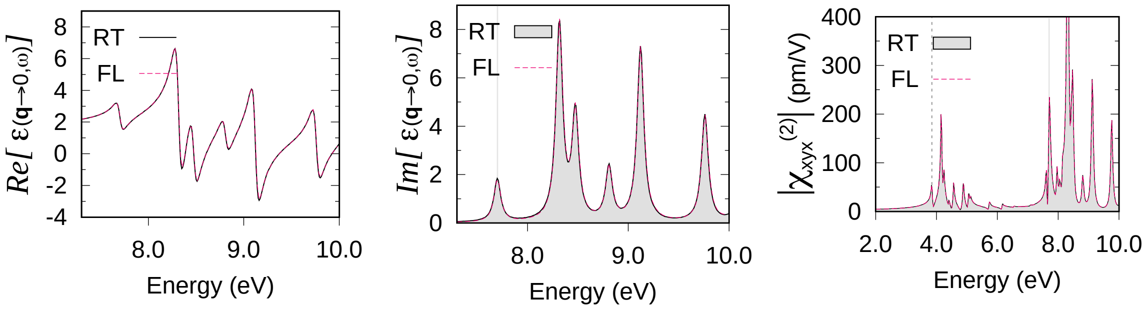


FIG. S34: h-BN 2D - 12×12×1 - small broadening

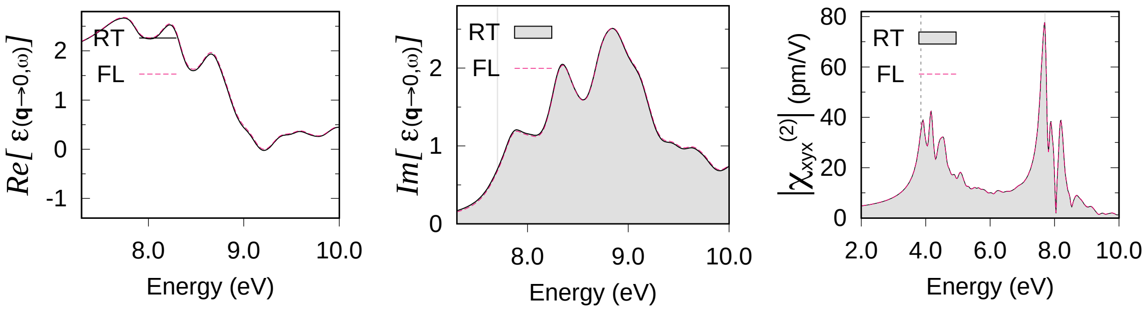


FIG. S35: h-BN 2D - 24×24×1 - large broadening

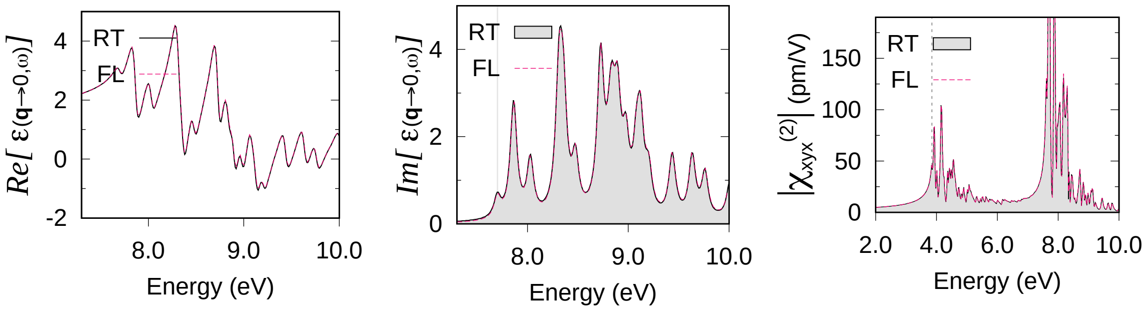


FIG. S36: h-BN 2D - 24×24×1 - small broadening

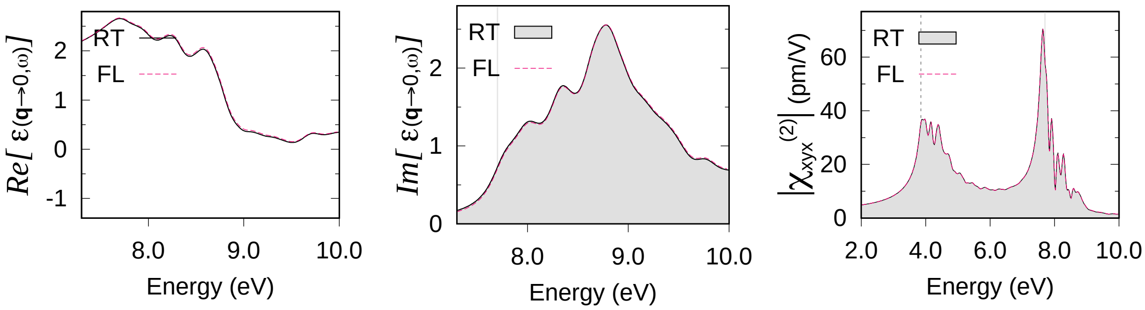


FIG. S37: h-BN 2D - 36×36×1 - large broadening

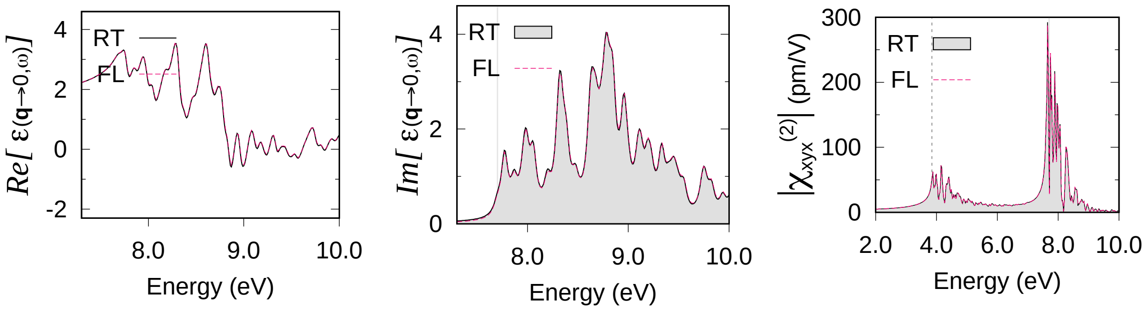


FIG. S38: h-BN 2D - 36×36×1 - small broadening

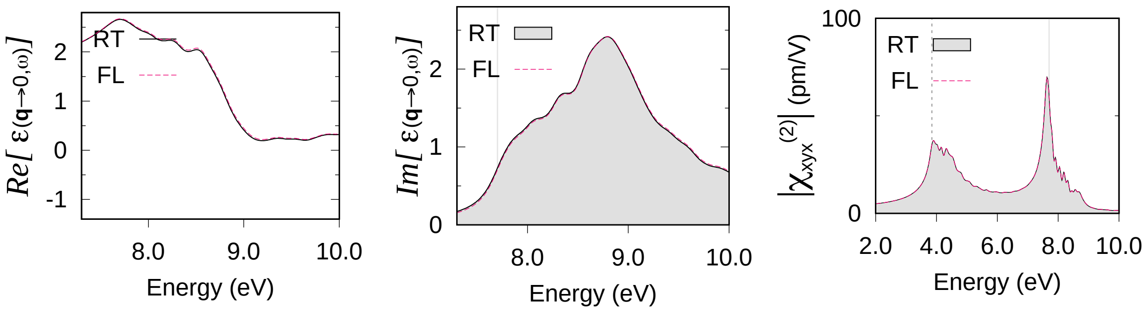


FIG. S39: h-BN 2D - 48×48×1 - large broadening

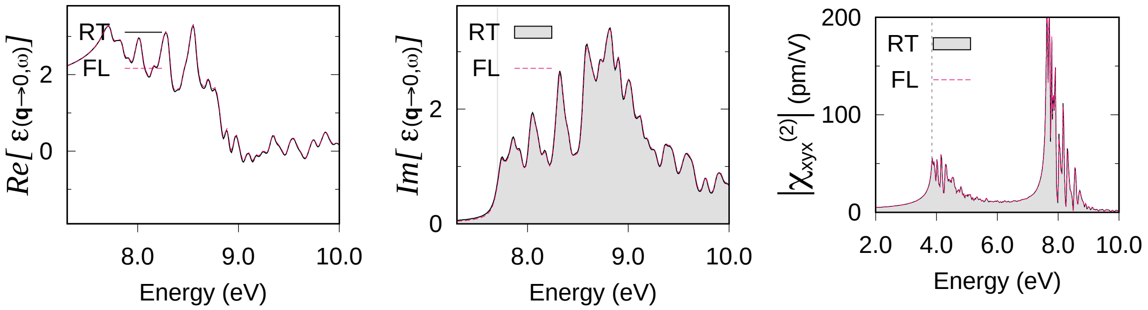


FIG. S40: h-BN 2D - 48×48×1 - small broadening

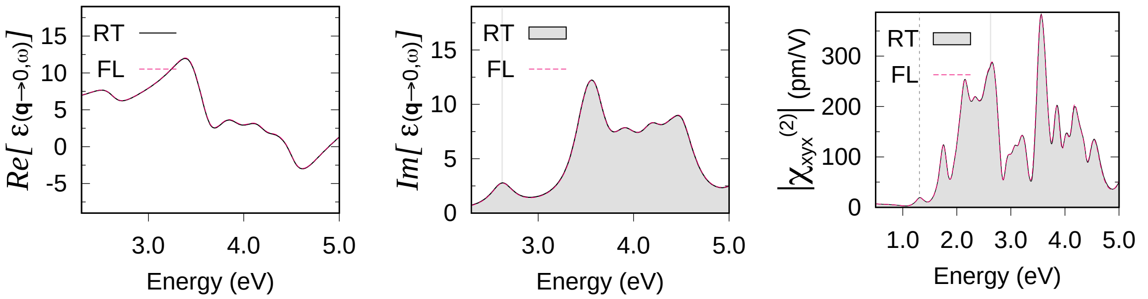


FIG. S41: $MoS_2$ 2D - 6×6×1 - large broadening

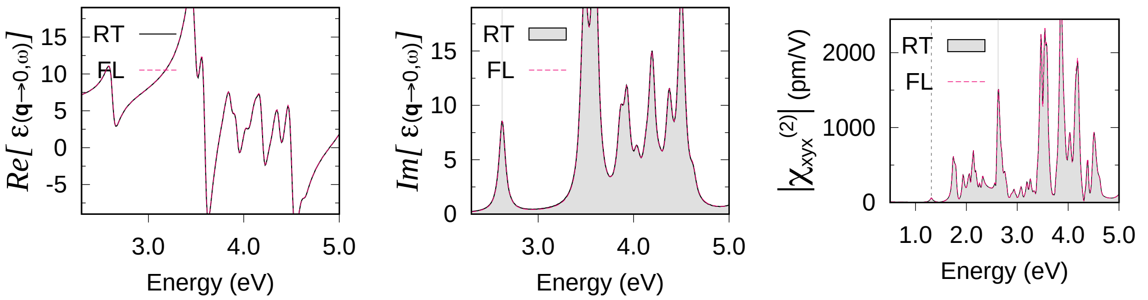


FIG. S42: $MoS_2$ 2D - 6×6×1 - small broadening

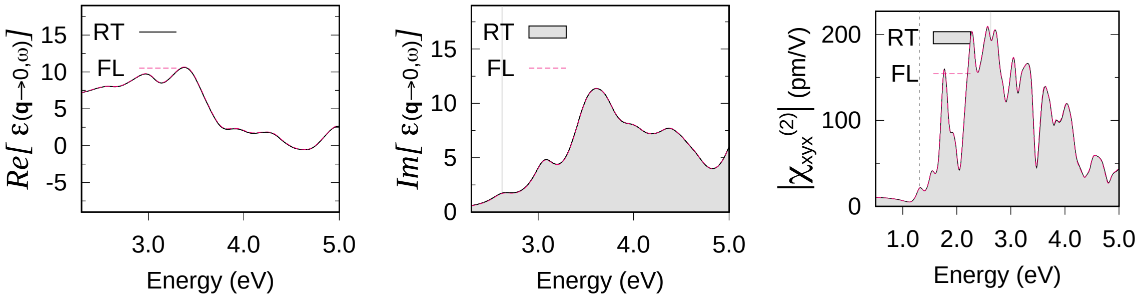


FIG. S43: $MoS_2$ 2D - 12×12×1 - large broadening

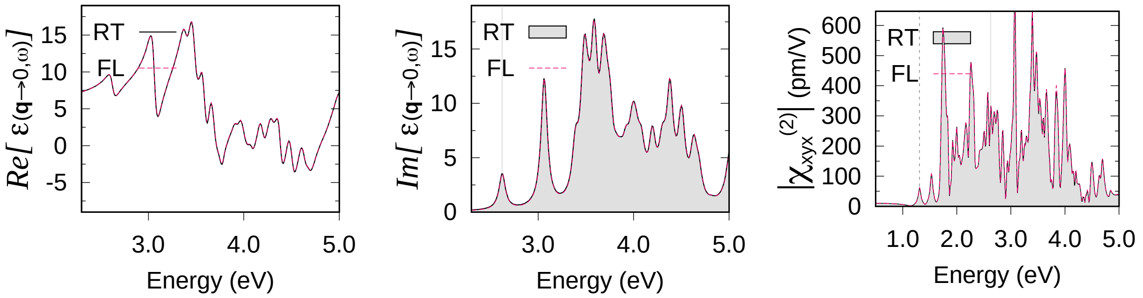


FIG. S44: $MoS_2$ 2D - 12×12×1 - small broadening

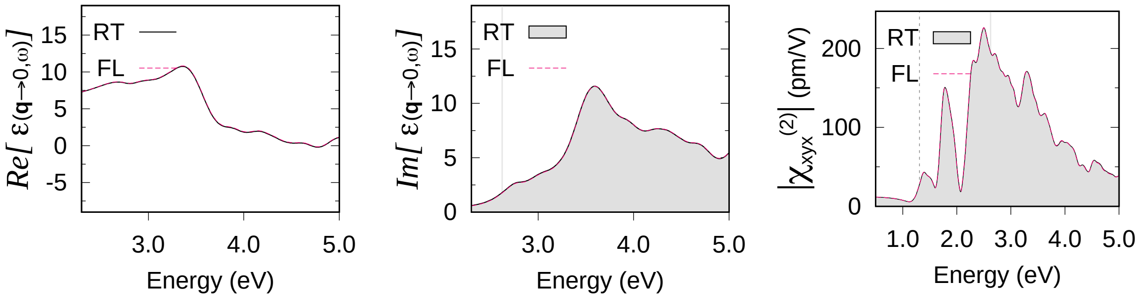


FIG. S45: $MoS_2$ 2D - 24×24×1 - large broadening

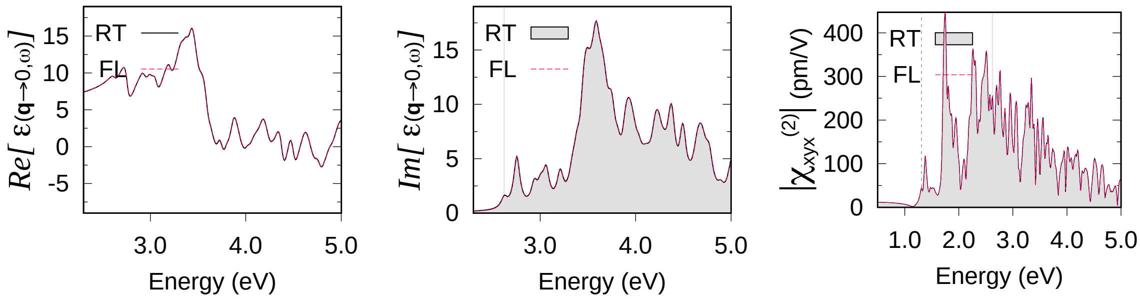


FIG. S46: $MoS_2$ 2D - 24×24×1 - small broadening

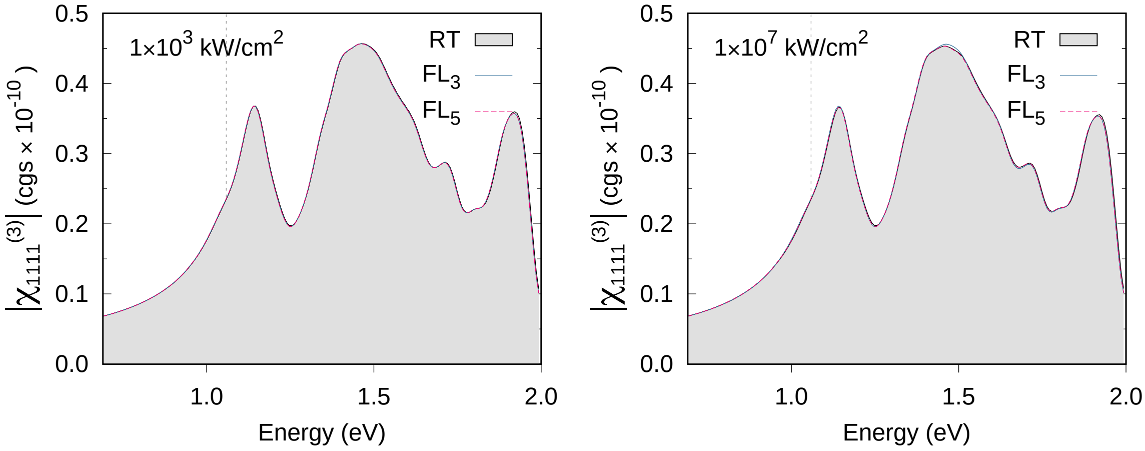


FIG. S47: Bulk Si THG - 8×8×8 - large broadening

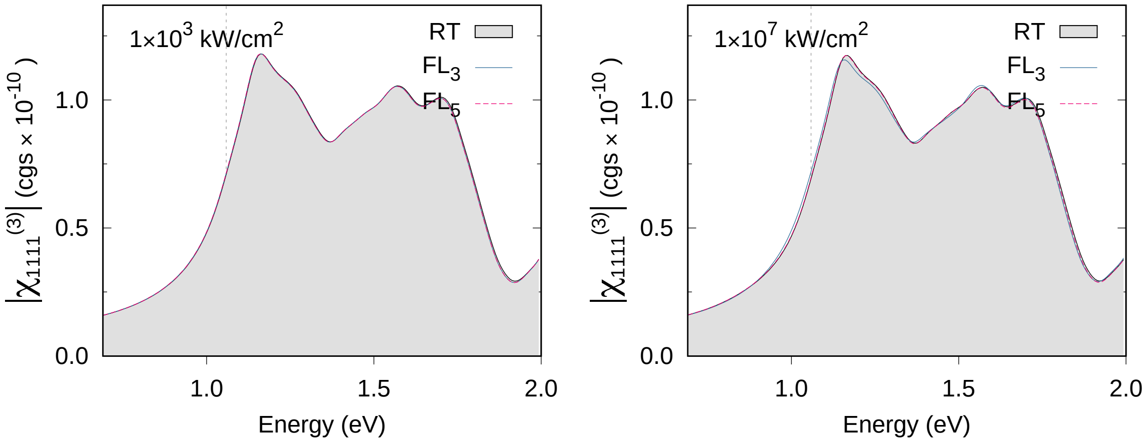


FIG. S48: Bulk Si THG - 24×24×24 - large broadening

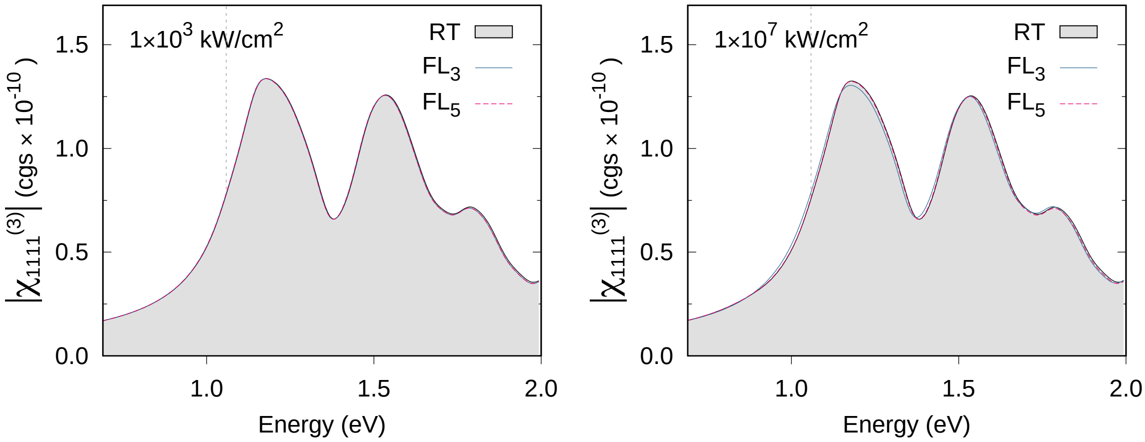


FIG. S49: Bulk Si THG - 32×32×32 - large broadening

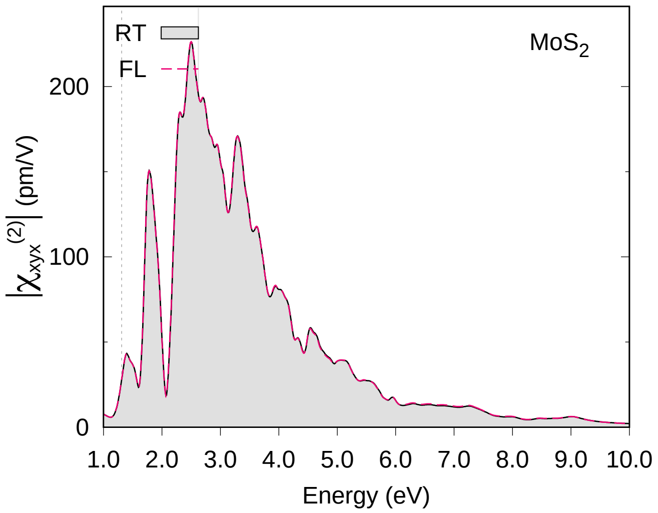


FIG. S50: $MoS_2$ 2D - 24×24×1 - large broadening - high energy range

## VII. CODE AND DATA AVAILABILITY

### A. Code availability

The Floquet approach developed in this work for calculating non-linear optical properties will be available in the next release of the Yambo code (Yambo 5.2). A tutorial will be made available in due course through the tutorials section (`http://www.yambo-code.org/wiki/index.php?title=Tutorials`) of the official Yambo website (`http://www.yambo-code.org/`).

### B. Data availability

Input and output files of the calculations presented in this study can be found in a GitHub repository (`https://github.com/aim137/Floquet_IPA-data_repository.git`).
